# Supplementary material for: Vickrey Auctions for Irregular Distributions
Source: arXiv:1306.4022 source file (2013-10-04)
Supplement: Supplementary file 1 [file appendix.tex]

\section{Targeted vs Non-targeted Advertising}\label{app:tvsnt}
Consider a population with two groups, and a single item auction among $n$ bidders for some niche good that appeals just to one group of the population,
which has a value of $n^2$ for the good. The other segment doesn't care much abotut the product. 
Specifically, suppose that the bidder valuations come from the following distribution, where the two cases represent
the two groups in the population. 
\begin{equation}
v_i=\begin{cases}
1 & \text{w.p. } 1-1/n^2\\
n^2 & \text{w.p. } 1/n^2
\end{cases}
\end{equation}
The optimal revenue for this setting is $\Theta(n)$. Consider running the Vickrey auction with a reserve price of $n^2$. 
The probability that at least one person exceeds the value of $n^2$ is roughly $1/n$. Thus the revenue is $\Omega(n)$. 

On the other hand, if we just ran the Vickrey auction, to get a good revenue we need at least two bidders to have values above $n^2$. If we add $k$ extra bidders from the same distribution as above, i.e. run a non-targeted advertising campaign we need a very large $k$ to get a good revenue. 

The probability that at least two bidders have a value above $n^2$ is $$\sum_{r=2}^{n+k}\binom{n+k}{r}\frac{1}{n^{2r}}(1-\frac{1}{n^2})^{n+k-r} \leq \sum_{r=2}^{n+k}\binom{n+k}{r}\frac{1}{n^{2r}}.$$ If this probability is $o(1/n)$, the revenue of Vickrey auction is $o(1/n)\cdot n^2 = o(n)$. To see the values of $k$ where this probability is $o(1/n)$, we have to consider the values of $k$ for which
$$\lim_{n\rightarrow \infty}\sum_{r=2}^{n+k}\binom{n+k}{r}\frac{1}{n^{2r-1}}$$
is zero. This quantity is a decreasing function of $r$, and thus it is enough to consider $r=2$. Clearly for $r=2$, if $k = o(n^{3/2})$, this quantity goes to zero. 
Thus, unless we add $\Theta(n^{3/2})$ bidders, Vickrey auction will have a revenue of just $o(n)$. On the other hand, just adding one extra bidder with value $1$ and one extra bidder with value $n^2$
gets higher revenue than the optimal revenue in the original setting. Though it is true that a bidder from the second group is very sparsely represented in the population, and hence
it is very difficult to recruit even one extra bidder from such a population, a targeted advertising campaign is still a far more effective means to boost revenue than a generic campaign. 

%\begin{proofof}{Corollary \ref{cor:vickrey}}
%Our main Lemma \ref{lem:commensurateExtension} states that the revenue of a Vickrey auction with one extra bidder from each group achieves
%at least $1/2$ of the optimal revenue without this extra bidder. Alternatively, one could view the above lemma in the opposite direction: The revenue
%of the Vickrey auction with $n_i$ bidders from each group achieves at least $1/2$ of the optimal revenue with $n_i-1$ bidders from each group. 
%
%Now we argue that the revenue of the optimal auction in the setting with $n_i-1$ bidders from each group is at least $\frac{\min_{i\in [k]}n_i-1}{\min_{i\in [k]}n_i}$ of the the optimal revenue with $n_i$ bidders from each group. The reason behind this is that the optimal auction can always be run in a way that it is symmetric for
%all bidders in the same group. Thereby the expected contribution of a bidder in group $i$ will be $\frac{1}{n_i}$. An auction for the setting with $n_i-1$
%bidders in each group is the following: Run the hypothetical optimal auction with one extra bidder in each group. Whenever the extra bidder is the winner
%just through him away. By doing so we are only losing a fraction of $\frac{1}{n_i}$ of the expected revenue contribution from each group of bidders. 
%Hence, this auction will achieve the desired revenue guarantee and thereby the optimal auction for the decreased bidder setting will also do so.
%\end{proofof}

\section{Deferred Proofs in Section~\ref{sec:dominant}}\label{app:dominant}
%We first prove a lemma for the regular distribution setting: bidders are drawn
%from a family of $k$ regular distributions such that one of them hazard-rate
%dominates the rest. This lemma can be extended to prove
%Theorem~\ref{thm:hazard-rate} in a manner identical to how Theorem 6.3 of
%Roughgarden et al.~\cite{RTY12} was extended to prove
%Theorem~\ref{thm:mainThm} in our paper. We don't repeat that extension here,
%and instead just prove the lemma. The lemma uses the notion of commensurate
%auctions defined by Hartline and Roughgarden~\cite{HR09}, which we define below:

\begin{defn}
An auction $M'$ is commensurate to $M$ if:
\begin{align}
\E[\phi_{W'}(v_{W'})|W'\neq W]\geq~& 0 \label{eq:com_1}\\
\E[\phi_{W}(v_{W})|W'\neq W]\leq~& \E_{\vals',\vals}[p_{W'}|W'\neq W] \label{eq:com_2}
\end{align} 
where $W',W$ are the winners of $M',M$ respectively and $p_{W'}$ is the
price paid by the winner of $M'$. 
\end{defn}

The lemma also uses a theorem from~\cite{HR09} which we state below and provide a proof for
completeness. 
\begin{theorem}[Hartline and Roughgarden~\cite{HR09}]
\label{thm:commensurate} If mechanism $M'$ is commensurate
to $M$ then $R_M \leq 2R_{M'}$
%\begin{align*}
%R_{M'}\geq \frac{1}{2}R_{M}
%\end{align*}
where $R_{M'}, R_M$ are the expected revenues of mechanisms $M'$ and $M$. 
\end{theorem}
\begin{proof}
By Myerson's characterization~\cite{M81} we know that the expected revenue of
any truthful auction is equal to its expected virtual surplus.
\begin{align*}
R_{M} =
\E[\phi_{W}(v_{W})]=~&\E[\phi_{W}(v_{W})|W'=W]Pr[W'=W]+\E[\phi_{W}(v_{W})|W'\neq
W]Pr[W'\neq W]\\
=~& \E[\phi_{W'}(v_{W'})|W'=W]Pr[W'=W]+\E[\phi_{W}(v_{W})|W'\neq W]Pr[W'\neq W]
\end{align*}
We lower bound each of the two terms in the RHS above by $R_{M'}$. By property \eqref{eq:com_1} we have:
\begin{align*}
&\E[\phi_{W'}(v_{W'})|W'=W]Pr[W'=W]\\
&\qquad\leq\E[\phi_{W'}(v_{W'})|W'=W]Pr[W'=W]+\E[\phi_{W'}(v_{W'})|W'\neq W]Pr[W'\neq W]\\
&\qquad=\E[\phi_{W'}(v_{W'})]=R_{M'}
\end{align*}
By property \eqref{eq:com_2} we have:
\begin{align*}
&\E[\phi_{W}(v_{W})|W'\neq W]Pr[W'\neq W]\\
&\qquad\leq \E[p_{W'}|W'\neq W]Pr[W'\neq W]\\
&\qquad\leq\E[p_{W'}|W'\neq W]Pr[W'\neq W]+\E[p_{W'}|W'= W]Pr[W'= W]=R_{M'}
\end{align*}
\end{proof}
